# Supplementary material for: Hamiltonian description of nonreciprocal interactions
Source: arXiv:2505.05246 source file (2026-06-16)
Supplement: Supplementary file 1 [file supp.tex]

% supp.tex
\newif\ifmainmode        \mainmodefalse
\newif\ifsuppmode         \suppmodetrue
\newif\ifcombinedmode \combinedmodefalse

\input{paper_body.tex}
